# Supplementary material for: Formulation of Relativistic Dissipative Spin Hydrodynamics
Source: arXiv:2512.20855 source file (2025-12-24)
Supplement: Supplementary file 1 [file appendixa.tex]

% From mitthesis package
% Version: 1.01, 2023/07/04
% Documentation: https://ctan.org/pkg/mitthesis

\chapter{Code listing}

\lstdefinestyle{mystyle}{
    backgroundcolor=\color{CadetBlue!15!white},   
    commentstyle=\color{Red3},
    numberstyle=\tiny\color{gray},
    stringstyle=\color{Blue3},
    basicstyle=\small\ttfamily,
    breakatwhitespace=false,         
    breaklines=true,                 
    numbers=left,                    
    numbersep=5pt,                  
    showspaces=false,                
    showstringspaces=false,
    showtabs=false,                  
    tabsize=2
}%
\lstset{language=[5.3]Lua,style={mystyle}}%

\begin{lstlisting}
function print_rate(kappa,xMin,xMax,npoints,option)
     local c = 1-kappa*kappa
     local croot = (1-kappa*kappa)^(1/2)
     local logx = math.log(xMin)
     local psi = 0
     
     local xstep = (math.log(xMax)-math.log(xMin))/(npoints-1)
     
     arg0 = math.sqrt(xMin/c)
     psi0 = (1/c)*math.exp((kappa*arg0)^2)*(erfc(kappa*arg0)-erfc(arg0))
     
     if option~=[[]] then
  		 tex.sprint("\\addplot+["..option.."] coordinates{") 
  		 -- addplot+ for color cycle to work
     else
  		 tex.sprint("\\addplot+ coordinates{")
     end
     tex.sprint("("..xMin..","..psi0..")")
     
     for i=1, (npoints-1) do
  		 x = math.exp(logx + xstep)
  		 arg = math.sqrt(x/c)
  		 karg = kappa*arg
  		 if karg<5 then 
		 -- this break compensates for exp(karg^2), which multiplies the error in the erf approximation...
  		    logpsi = -math.log(croot) + karg^2 + math.log(erfc(karg)-erfc(arg))
  		    psi = math.exp(logpsi)
  		 else
  		    psi = (1/(karg) - 1/(2*(karg^3)) + 3/(4*(arg^5)) )/(1.77245385*croot)
  		    -- this is the large x asymptote of the reaction rate
  		 end
  		 logx = math.log(x)
  		 tex.sprint("("..x..","..psi..")")
     end
     tex.sprint("}")
end
\end{luacode*}
\end{lstlisting}
